# Supplementary material for: Performance of Automatic Active Space Selection for Electronic Excitation Energies
Source: arXiv:2511.05732 source file (2025-11-18)
Supplement: Supplementary file 1 [file SI.pdf]

## Supporting information: active spaces, excitation energies and reference data

NEVPT2

Active space size

| | ASF(S) | I-ASF(S) | ASF(T) | I-ASF(T) | ASF(QRO) | I-ASF(QRO) |
|---|---|---|---|---|---|---|
| acetamide | (8, 7) | (8, 7) | (4, 4) | (4, 4) | (4, 4) | (4, 4) |
| adenine | (8, 8) | (10, 9) | (8, 8) | (8, 8) | (10, 9) | (12, 10) |
| benzoquinone | (16, 12) | (16, 12) | (8, 8) | (8, 8) | (8, 8) | (14, 11) |
| cyclopentadiene | (4, 4) | (8, 8) | (4, 4) | (4, 4) | (4, 4) | (8, 8) |
| cyclopropene | (4, 4) | (10, 10) | (6, 5) | (6, 5) | (4, 4) | (4, 4) |
| cytosine | (6, 6) | (8, 7) | (8, 7) | (8, 7) | (6, 6) | (10, 8) |
| formamide | (8, 7) | (8, 7) | (6, 6) | (6, 6) | (4, 4) | (4, 4) |
| hexatriene | (6, 6) | (6, 6) | (6, 6) | (6, 6) | (6, 6) | (6, 6) |
| norbornadiene | (6, 5) | (6, 5) | (4, 4) | (4, 4) | (6, 5) | (6, 5) |
| octatetraene | (8, 8) | (8, 8) | (8, 8) | (8, 8) | (8, 8) | (8, 8) |
| propanamide | (8, 5) | (8,5) | (4, 4) | (4, 4) | (4, 4) | (4, 4) |
| pyrrole | (6, 5) | (6, 5) | (6, 5) | (6, 5) | (6, 5) | (6, 5) |
| thymine | (8, 7) | (10, 8) | (8, 7) | (8, 7) | (8, 7) | (8, 7) |
| triazine | (6, 6) | (10, 10) | (10, 8) | (10, 8) | (10, 8) | (10, 8) |
| uracil | (10, 8) | (12, 10) | (18, 12) | (18, 12) | (8, 7) | (8, 7) |
| acetaldehyde | (8, 6) | (8, 7) | (4, 3) | (8, 8) | (4, 3) | (10, 9) |
| acetone | (8, 7) | (8, 7) | (4, 3) | (10, 9) | (4, 3) | (4, 3) |
| benzene | (6, 6) | (6, 6) | (6, 6) | (6, 6) | (6, 6) | (6, 6) |
| butadiene | (4, 4) | (4, 4) | (4, 4) | (6, 6) | (4, 4) | (4, 4) |
| DMABN | (12, 12) | (12, 12) | (12, 12) | (14, 13) | (14, 13) | (14, 13) |
| ethylene | (4, 3) | (6, 5) | (4, 3) | (8, 8) | (4, 3) | (4, 3) |
| formaldehyde | (8, 7) | (8, 7) | (4, 3) | (8, 7) | (4, 3) | (6, 5) |
| furan | (8, 7) | (8, 7) | (4, 4) | (4, 4) | (6, 5) | (6, 5) |
| hexatriene | (6, 6) | (6, 6) | (6, 6) | (6, 6) | (6, 6) | (6, 6) |
| naphthalene | (10, 10) | (10, 10) | (10, 10) | (10, 10) | (10, 10) | (10, 10) |
| pNA | (8, 8) | (12, 11) | (8, 8) | (12, 11) | (8, 8) | (14, 12) |
| pyrazine | (6, 6) | (8, 8) | (10, 8) | (10, 8) | (10, 8) | (10, 8) |
| pyridazine | (6, 5) | (14, 11) | (10, 8) | (10, 9) | (10, 8) | (10, 8) |
| pyridine | (6, 6) | (6, 6) | (6, 6) | (6, 6) | (6, 6) | (6, 6) |
| pyrimidine | (12, 9) | (14, 11) | (10, 9) | (10, 9) | (8, 7) | (6, 6) |
| stetrazine | (10, 8) | (18, 15) | (10, 8) | (16, 15) | (12, 9) | (16, 14) |
| water | (6, 6) | (6, 6) | (4, 5) | (4, 5) | (4, 5) | (4, 5) |

NEVPT2

Excitation energy

| | ASF(S) | I-ASF(S) | ASF(T) | I-ASF(T) | ASF(QRO) | I-ASF(QRO) |
|---|---|---|---|---|---|---|
| acetamide | 5.64343345 | 5.64330467 | 7.09280837 | 7.09280837 | 7.09275634 | 7.09273819 |
| adenine | 5.65613128 | 5.5889308 | 5.65624156 | 5.65624156 | 5.58898461 | 5.48635054 |
| benzoquinone | 4.36836036 | 4.36830639 | 4.33419831 | 4.33419831 | 4.33417706 | 4.36119318 |
| cyclopentadiene | 6.77158965 | 5.54055804 | 6.77146649 | 6.77146649 | 6.77148616 | 6.72892849 |
| cyclopropene | 6.77423432 | 6.85655922 | | 0 | 6.77422649 | 6.77412997 |
| cytosine | 4.81346222 | 4.72733609 | 4.72734706 | 4.72734706 | 4.81328299 | 4.75817179 |
| formamide | 5.5499178 | 5.54991731 | 7.18006095 | 7.18006095 | 7.30203618 | 7.30203617 |
| hexatriene | 5.58893002 | 5.58889384 | 5.58890202 | 5.58890202 | 5.58888908 | 5.58890346 |
| norbornadiene | | 5.16117957 | 5.20600538 | 5.20600538 | | 5.16623861 |
| octatetraene | 4.73519275 | 4.73519182 | 4.73519463 | 4.73519463 | 4.73518958 | 4.73519366 |
| propanamide | | | 7.07547171 | 7.07547171 | 7.07542731 | 7.07542724 |
| pyrrole | 6.59308169 | 6.59310072 | 6.59310243 | 6.59310243 | 6.59313402 | 6.59313453 |
| thymine | 5.21685939 | 5.15543352 | 5.2168842 | 5.2168842 | 5.21691264 | 5.21693238 |
| triazine | 6.03980451 | 5.90794876 | 4.91331475 | 4.91331475 | 4.9132483 | 4.91326429 |
| uracil | 5.29283054 | 5.36507066 | | | 5.37743657 | 5.37742944 |
| acetaldehyde | 4.31900153 | 4.30609937 | 4.47071467 | 4.41232421 | 4.47071006 | 4.4267007 |
| acetone | 4.47929092 | 4.47929213 | 4.6164652 | 4.53809473 | 4.6164366 | 4.61647788 |
| benzene | 5.22424248 | 5.22480494 | 5.22487716 | 5.2241681 | 5.22460946 | 5.22475642 |
| butadiene | 6.80949154 | 6.80949038 | 6.80955244 | 6.83140441 | 6.80956129 | 6.80956068 |
| DMABN | 3.81244456 | 3.81244449 | 3.81245251 | 3.65928598 | 3.66003144 | 3.65966007 |
| ethylene | 8.01458156 | 8.03493114 | 8.00414935 | 8.08769267 | 8.0044892 | 8.00450239 |
| formaldehyde | 3.95491066 | 3.95490704 | 4.15333256 | 3.95490909 | 4.15334615 | 3.97657275 |
| furan | 6.7812056 | 6.78120808 | 6.83143236 | 6.83143236 | 6.76845178 | 6.76845178 |
| hexatriene | 5.59375104 | 5.5937216 | 5.59372902 | 5.59373827 | 5.59372462 | 5.59369869 |
| naphthalene | 4.42716715 | 4.42693123 | 4.4269286 | 4.42692749 | 4.42693897 | 4.42693902 |
| pNA | 5.05740307 | 5.07146102 | 5.05740153 | 5.07140728 | 5.0573919 | 5.06908231 |
| pyrazine | 5.28256734 | 5.22131375 | 4.21421431 | 4.21422204 | 4.21423722 | 4.21420643 |
| pyridazine | 5.85469816 | | 3.83124125 | 4.32885957 | 3.83118508 | 3.83121273 |
| pyridine | 5.3952249 | 5.39522658 | 5.39528588 | 5.39528665 | 5.39518559 | 5.39518506 |
| pyrimidine | 5.65162169 | 5.58535052 | 5.08914791 | 5.08899139 | 5.11252487 | 5.06943752 |
| stetrazine | 2.67861156 | | 2.3364637 | 3.28391198 | 2.42235772 | 2.65987127 |
| water | 9.47067101 | 9.47066676 | 7.60250067 | 7.60250097 | 7.6025048 | 7.60249942 |

Reference Excitation values

| | |
|---|---|
| acetamide | 5.8 |
| adenine | 5.2 |
| benzoquinone | 2.8 |
| cyclopentadiene | 5.51 |
| cyclopropene | 6.76 |
| cytosine | 4.68 |
| formamide | 5.63 |
| hexatriene | 5.31 |
| norbornadiene | 5.34 |
| octatetraene | 4.64 |
| propanamide | 5.72 |
| pyrrole | 6.31 |
| thymine | 4.94 |
| triazine | 6.31 |
| uracil | 4.9 |
| acetaldehyde | 4.27 |
| acetone | 4.44 |
| benzene | 4.99 |
| butadiene | 6.38 |
| DMABN | 4.87 |
| ethylene | 8.16 |
| formaldehyde | 3.92 |
| furan | 6.32 |
| hexatriene | 5.32 |
| naphthalene | 4.24 |
| pNA | 4.62 |
| pyrazine | 4.04 |
| pyridazine | 3.67 |
| pyridine | 5.06 |
| pyrimidine | 4.38 |
| stetrazine | 2.56 |
| water | 7.61 |
